# Supplementary material for: First Place Solution to the ECCV 2024 BRAVO Challenge: Evaluating Robustness of Vision Foundation Models for Semantic Segmentation
Source: arXiv:2409.17208 source file (2024-10-08)
Supplement: Supplementary file 1 [file suppl.tex]

\clearpage
\setcounter{page}{1}
\maketitlesupplementary
